# Supplementary material for: Discovery of a Gamma-ray Black Widow Pulsar by GPU-accelerated Einstein@Home
Source: arXiv:2009.01513 ancillary file (2020-10-22)
Supplement: Supplementary file 1 [file supp_paper_J1653.pdf]

## Discovery of a Gamma-ray Black Widow Pulsar by GPU-accelerated Einstein@Home Supplementary Material

L. NIEDER 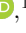<sup>1,2</sup> C. J. CLARK 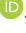<sup>3</sup> D. KANDEL 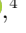<sup>4</sup> R. W. ROMANI 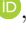<sup>4</sup> C. G. BASSA 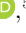<sup>5</sup> B. ALLEN 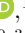<sup>1,6,2</sup> A. ASHOK 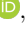<sup>1,2</sup>  
I. COGNARD 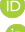<sup>7,8</sup> H. FEHRMANN 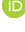<sup>1,2</sup> P. FREIRE 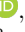<sup>9</sup> R. KARUPPUSAMY 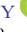<sup>9</sup> M. KRAMER 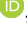<sup>9,3</sup> D. LI 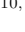<sup>10,11</sup>  
B. MACHENSCHALK 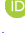<sup>1,2</sup> Z. PAN 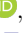<sup>10</sup> M. A. PAPA 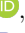<sup>1,6,2</sup> S. M. RANSOM 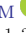<sup>12</sup> P. S. RAY 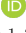<sup>13</sup> J. ROY 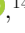<sup>14</sup> P. WANG 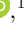<sup>10</sup>  
J. WU 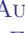<sup>9</sup> C. AULBERT 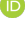<sup>1,2</sup> E. D. BARR 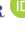<sup>9</sup> B. BEHESHTIPOUR 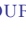<sup>1,2</sup> O. BEHNKE 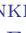<sup>1,2</sup> B. BHATTACHARYYA 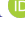<sup>14</sup>  
R. P. BRETON 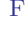<sup>3</sup> F. CAMILO 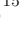<sup>15</sup> C. CHOQUET 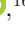<sup>16</sup> V. S. DHILLON 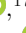<sup>17,18</sup> E. C. FERRARA 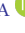<sup>19,20</sup> L. GUILLEMOT 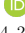<sup>7,8</sup>  
J. W. T. HESSELS 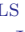<sup>5,21</sup> M. KERR 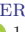<sup>13</sup> S. A. KWANG 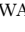<sup>22</sup> T. R. MARSH 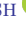<sup>23</sup> M. B. MICKALIGER 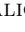<sup>3</sup> Z. PLEUNIS 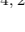<sup>24,25</sup>  
H. J. PLETSCH 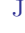<sup>1</sup> M. S. E. ROBERTS 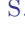<sup>26,27</sup> S. SANPA-ARSA 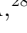<sup>28</sup> AND B. STELTNER 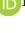<sup>1,2</sup>

<sup>1</sup>Max-Planck-Institut für Gravitationsphysik (Albert-Einstein-Institut), 30167 Hannover, Germany

<sup>2</sup>Leibniz Universität Hannover, 30167 Hannover, Germany

<sup>3</sup>Jodrell Bank Centre for Astrophysics, Department of Physics and Astronomy, The University of Manchester, M13 9PL, UK

<sup>4</sup>KIPAC/Dept. of Physics, Stanford University, Stanford, CA 94305, USA

<sup>5</sup>ASTRON, The Netherlands Institute for Radio Astronomy, Oude Hoogeveensedijk 4, 7991 PD Dwingeloo, The Netherlands

<sup>6</sup>Department of Physics, University of Wisconsin–Milwaukee, P.O. Box 413, Milwaukee, WI 53201, USA

<sup>7</sup>Laboratoire de Physique et Chimie de l'Environnement et de l'Espace, Université d'Orléans / CNRS, F-45071 Orléans Cedex 02, France

<sup>8</sup>Station de radioastronomie de Nançay, Observatoire de Paris, CNRS/INSU, F-18330 Nançay, France

<sup>9</sup>Max-Planck-Institut für Radioastronomie, auf dem Hügel 69, 53121 Bonn, Germany

<sup>10</sup>National Astronomical Observatories, Chinese Academy of Sciences, Beijing 100101, China

<sup>11</sup>NAOC-UKZN Computational Astrophysics Centre, University of KwaZulu-Natal, Durban 4000, South Africa

<sup>12</sup>National Radio Astronomy Observatory, 520 Edgemont Rd., Charlottesville, VA USA 22903

<sup>13</sup>Space Science Division, Naval Research Laboratory, Washington, DC 20375-5352, USA

<sup>14</sup>National Centre for Radio Astrophysics, Tata Institute of Fundamental Research, Pune 411 007, India

<sup>15</sup>South African Radio Astronomy Observatory, 2 Fir Street, Black River Park, Observatory 7925, South Africa

<sup>16</sup>Résidence Le Dauphiné, rue Jean Bleuzen, Vanves, France

<sup>17</sup>Department of Physics and Astronomy, University of Sheffield, Sheffield S3 7RH, UK

<sup>18</sup>Instituto de Astrofísica de Canarias, E-38205 La Laguna, Tenerife, Spain

<sup>19</sup>NASA Goddard Space Flight Center, Greenbelt, MD 20771, USA

<sup>20</sup>Department of Astronomy, University of Maryland, College Park, MD 20742, USA

<sup>21</sup>Anton Pannekoek Institute for Astronomy, University of Amsterdam, Science Park 904, 1098 XH Amsterdam, The Netherlands

<sup>22</sup>Department of Physics, University of Wisconsin–Milwaukee, P.O. Box 413, Milwaukee, WI 53201, USA

<sup>23</sup>Astronomy and Astrophysics Group, Department of Physics, University of Warwick, Coventry CV4 7AL, UK

<sup>24</sup>Department of Physics, McGill University, 3600 rue University, Montréal, QC H3A 2T8, Canada

<sup>25</sup>McGill Space Institute, McGill University, 3550 rue University, Montréal, QC H3A 2A7, Canada

<sup>26</sup>New York University Abu Dhabi, P.O. Box 129188, Abu Dhabi, UAE

<sup>27</sup>Eureka Scientific, Inc. 2452 Delmer Street, Suite 100, Oakland, CA 94602-3017, USA

<sup>28</sup>National Astronomical Research Institute of Thailand (Public Organization), 260 Moo 4, T. Donkaew, A. Maerim, Chiang Mai, 50180, Thailand

(Received 2020 September 1; Revised 2020 September 22; Accepted 2020 September 25; Published 2020 October 22)

### CONTINUOUS GRAVITATIONAL WAVES

Acknowledging the possibility of mismatches between the pulsar rotation frequency and the gravitational-wave frequency, we perform an  $\mathcal{F}$ -statistic search in

a  $\sim 2$  Hz band around twice the rotation frequency, a factor of  $10^{-3}$  of the gravitational-wave frequency, similarly to what was done in [Abbott et al. \(2019\)](#) and also extend the spin-down search to the range  $2\dot{f} \in (-1.260, -1.2216) \times 10^{-15} \text{ Hz s}^{-1}$ . Overall, we use  $2.4 \times 10^9$  templates resulting in an average mismatch of 1%. We examine the results in 10 mHz-wide bands. The most significant  $2\mathcal{F}$  values from each band are consistent with the noise-only expectation, apart from six

outliers that can be ascribed to a disturbance in L1 around  $\approx 1016.32$  Hz. We set upper limits in each band. The values are plotted in Figure 1. The mean value is  $1.3 \times 10^{-25}$  and it is higher than the targeted search upper limit, consistently with the larger volume of searched wave shapes.

**Table 1.** Upper limits on  $h_0^{95\%}$  in each of the 10 mHz bands.

| Start freq. (Hz) | $h_0^{95\%} \times 10^{-25}$ |
|------------------|------------------------------|
| 1015.408         | $1.34^{+0.25}_{-0.23}$       |
| 1015.418         | $1.23^{+0.22}_{-0.23}$       |
| 1015.428         | $1.36^{+0.27}_{-0.26}$       |
| 1015.438         | $1.3^{+0.26}_{-0.24}$        |
| 1015.448         | $1.3^{+0.24}_{-0.24}$        |
| 1015.458         | $1.33^{+0.25}_{-0.23}$       |
| 1015.468         | $1.26^{+0.24}_{-0.23}$       |
| 1015.478         | $1.42^{+0.27}_{-0.25}$       |
| 1015.488         | $1.4^{+0.26}_{-0.25}$        |
| 1015.498         | $1.35^{+0.26}_{-0.25}$       |
| 1015.508         | $1.31^{+0.25}_{-0.23}$       |
| 1015.518         | $1.34^{+0.28}_{-0.27}$       |
| 1015.528         | $1.48^{+0.29}_{-0.28}$       |
| 1015.538         | $1.35^{+0.27}_{-0.25}$       |
| 1015.548         | $1.22^{+0.21}_{-0.22}$       |
| 1015.558         | $1.41^{+0.28}_{-0.26}$       |
| 1015.568         | $1.36^{+0.26}_{-0.24}$       |
| 1015.578         | $1.28^{+0.26}_{-0.25}$       |
| 1015.588         | $1.26^{+0.23}_{-0.22}$       |
| 1015.598         | $1.35^{+0.26}_{-0.24}$       |
| 1015.608         | $1.29^{+0.24}_{-0.24}$       |
| 1015.618         | $1.35^{+0.26}_{-0.24}$       |
| 1015.628         | $1.35^{+0.29}_{-0.28}$       |
| 1015.638         | $1.28^{+0.24}_{-0.22}$       |
| 1015.648         | $1.25^{+0.23}_{-0.22}$       |
| 1015.658         | $1.26^{+0.24}_{-0.23}$       |
| 1015.668         | $1.25^{+0.22}_{-0.23}$       |
| 1015.678         | $1.23^{+0.23}_{-0.23}$       |
| 1015.688         | $1.2^{+0.21}_{-0.22}$        |
| 1015.698         | $1.3^{+0.25}_{-0.23}$        |
| 1015.708         | $1.32^{+0.26}_{-0.24}$       |
| 1015.718         | $1.23^{+0.28}_{-0.3}$        |
| 1015.728         | $1.3^{+0.25}_{-0.23}$        |
| 1015.738         | $1.26^{+0.23}_{-0.22}$       |

**Table 1** *continued*

**Table 1** (*continued*)

| Start freq. (Hz) | $h_0^{95\%} \times 10^{-25}$ |
|------------------|------------------------------|
| 1015.748         | $1.4^{+0.26}_{-0.25}$        |
| 1015.758         | $1.23^{+0.22}_{-0.23}$       |
| 1015.768         | $1.41^{+0.26}_{-0.24}$       |
| 1015.778         | $1.27^{+0.31}_{-0.33}$       |
| 1015.788         | $1.34^{+0.26}_{-0.24}$       |
| 1015.798         | $1.22^{+0.29}_{-0.32}$       |
| 1015.808         | $1.21^{+0.21}_{-0.22}$       |
| 1015.818         | $1.23^{+0.21}_{-0.21}$       |
| 1015.828         | $1.32^{+0.25}_{-0.24}$       |
| 1015.838         | $1.23^{+0.21}_{-0.21}$       |
| 1015.848         | $1.21^{+0.22}_{-0.23}$       |
| 1015.858         | $1.47^{+0.29}_{-0.27}$       |
| 1015.868         | $1.29^{+0.25}_{-0.23}$       |
| 1015.878         | $1.28^{+0.24}_{-0.23}$       |
| 1015.888         | $1.29^{+0.25}_{-0.24}$       |
| 1015.898         | $1.32^{+0.24}_{-0.24}$       |
| 1015.908         | $1.27^{+0.23}_{-0.22}$       |
| 1015.918         | $1.29^{+0.24}_{-0.24}$       |
| 1015.928         | $1.44^{+0.29}_{-0.27}$       |
| 1015.938         | $1.2^{+0.21}_{-0.22}$        |
| 1015.948         | $1.24^{+0.22}_{-0.22}$       |
| 1015.958         | $1.27^{+0.23}_{-0.22}$       |
| 1015.968         | $1.26^{+0.23}_{-0.23}$       |
| 1015.978         | $1.2^{+0.21}_{-0.23}$        |
| 1015.988         | $1.38^{+0.27}_{-0.25}$       |
| 1015.998         | $1.29^{+0.26}_{-0.24}$       |
| 1016.008         | $1.27^{+0.24}_{-0.23}$       |
| 1016.018         | $1.27^{+0.24}_{-0.23}$       |
| 1016.028         | $1.37^{+0.27}_{-0.25}$       |
| 1016.038         | $1.24^{+0.21}_{-0.21}$       |
| 1016.048         | $1.24^{+0.23}_{-0.23}$       |
| 1016.058         | $1.32^{+0.26}_{-0.25}$       |
| 1016.068         | $1.4^{+0.26}_{-0.25}$        |
| 1016.078         | $1.39^{+0.28}_{-0.26}$       |
| 1016.088         | $1.33^{+0.26}_{-0.25}$       |
| 1016.098         | $1.4^{+0.27}_{-0.26}$        |
| 1016.108         | $1.26^{+0.23}_{-0.23}$       |
| 1016.118         | $1.31^{+0.25}_{-0.24}$       |
| 1016.128         | $1.35^{+0.26}_{-0.24}$       |
| 1016.138         | $1.28^{+0.25}_{-0.23}$       |
| 1016.148         | $1.2^{+0.21}_{-0.22}$        |

**Table 1** *continued*

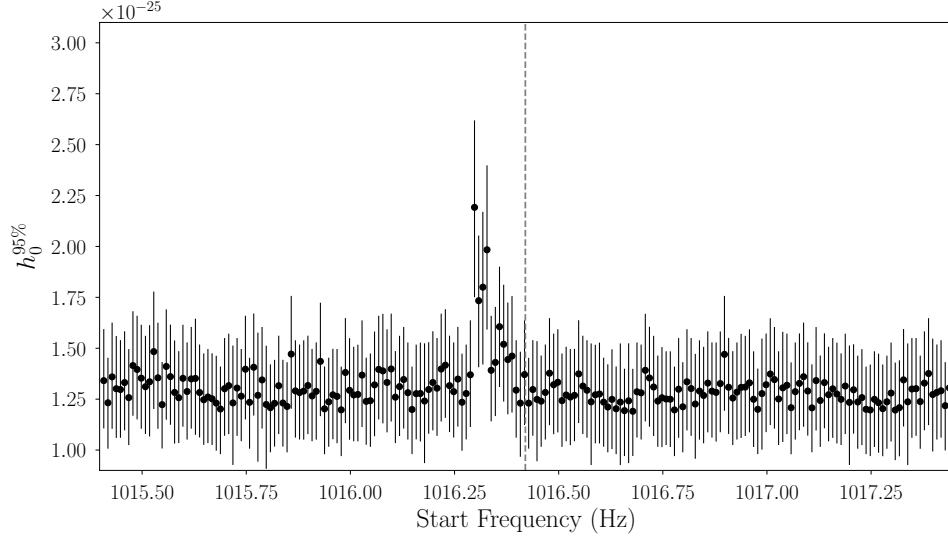

**Figure 1.** 95% confidence upper limits on the gravitational-wave amplitude in 10 mHz bands around twice the rotation frequency of PSR J1653–0158, which is indicated by the gray dashed line. The bars indicate a conservative estimate of the uncertainty on the upper limit values. The “spike” does not indicate a detection: it is due to a disturbance in L1 around  $\approx 1016.32$  Hz.

**Table 1** (*continued*)

| Start freq. (Hz) | $h_0^{95\%} \times 10^{-25}$ |
|------------------|------------------------------|
| 1016.158         | $1.28^{+0.24}_{-0.22}$       |
| 1016.168         | $1.28^{+0.25}_{-0.24}$       |
| 1016.178         | $1.24^{+0.28}_{-0.3}$        |
| 1016.188         | $1.3^{+0.23}_{-0.22}$        |
| 1016.198         | $1.33^{+0.25}_{-0.23}$       |
| 1016.208         | $1.3^{+0.25}_{-0.23}$        |
| 1016.218         | $1.4^{+0.27}_{-0.26}$        |
| 1016.228         | $1.42^{+0.27}_{-0.26}$       |
| 1016.238         | $1.32^{+0.25}_{-0.23}$       |
| 1016.248         | $1.29^{+0.24}_{-0.23}$       |
| 1016.258         | $1.35^{+0.26}_{-0.23}$       |
| 1016.268         | $1.23^{+0.24}_{-0.24}$       |
| 1016.278         | $1.28^{+0.24}_{-0.23}$       |
| 1016.288         | $1.37^{+0.27}_{-0.26}$       |
| 1016.298         | $2.19^{+0.43}_{-0.44}$       |
| 1016.308         | $1.73^{+0.32}_{-0.33}$       |
| 1016.318         | $1.8^{+0.37}_{-0.38}$        |
| 1016.328         | $1.98^{+0.41}_{-0.39}$       |
| 1016.338         | $1.39^{+0.27}_{-0.25}$       |
| 1016.348         | $1.43^{+0.27}_{-0.26}$       |
| 1016.358         | $1.61^{+0.29}_{-0.3}$        |
| 1016.368         | $1.52^{+0.29}_{-0.28}$       |
| 1016.378         | $1.44^{+0.28}_{-0.27}$       |

**Table 1** *continued*

**Table 1** (*continued*)

| Start freq. (Hz) | $h_0^{95\%} \times 10^{-25}$ |
|------------------|------------------------------|
| 1016.388         | $1.46^{+0.29}_{-0.28}$       |
| 1016.398         | $1.29^{+0.25}_{-0.23}$       |
| 1016.408         | $1.23^{+0.25}_{-0.26}$       |
| 1016.418         | $1.37^{+0.27}_{-0.25}$       |
| 1016.428         | $1.23^{+0.22}_{-0.22}$       |
| 1016.438         | $1.3^{+0.24}_{-0.23}$        |
| 1016.448         | $1.25^{+0.29}_{-0.3}$        |
| 1016.458         | $1.24^{+0.22}_{-0.22}$       |
| 1016.468         | $1.28^{+0.24}_{-0.23}$       |
| 1016.478         | $1.38^{+0.27}_{-0.26}$       |
| 1016.488         | $1.32^{+0.25}_{-0.24}$       |
| 1016.498         | $1.33^{+0.26}_{-0.25}$       |
| 1016.508         | $1.24^{+0.23}_{-0.23}$       |
| 1016.518         | $1.27^{+0.24}_{-0.23}$       |
| 1016.528         | $1.26^{+0.24}_{-0.24}$       |
| 1016.538         | $1.27^{+0.23}_{-0.23}$       |
| 1016.548         | $1.37^{+0.26}_{-0.24}$       |
| 1016.558         | $1.31^{+0.25}_{-0.24}$       |
| 1016.568         | $1.29^{+0.25}_{-0.23}$       |
| 1016.578         | $1.24^{+0.29}_{-0.31}$       |
| 1016.588         | $1.27^{+0.25}_{-0.24}$       |
| 1016.598         | $1.28^{+0.25}_{-0.24}$       |
| 1016.608         | $1.24^{+0.22}_{-0.22}$       |

**Table 1** *continued*

**Table 1** (*continued*)

| Start freq. (Hz) | $h_0^{95\%} \times 10^{-25}$ |
|------------------|------------------------------|
| 1016.618         | $1.21^{+0.21}_{-0.22}$       |
| 1016.628         | $1.25^{+0.25}_{-0.24}$       |
| 1016.638         | $1.2^{+0.21}_{-0.22}$        |
| 1016.648         | $1.24^{+0.29}_{-0.31}$       |
| 1016.658         | $1.19^{+0.21}_{-0.22}$       |
| 1016.668         | $1.24^{+0.28}_{-0.31}$       |
| 1016.678         | $1.19^{+0.21}_{-0.22}$       |
| 1016.688         | $1.29^{+0.24}_{-0.22}$       |
| 1016.698         | $1.28^{+0.24}_{-0.23}$       |
| 1016.708         | $1.39^{+0.28}_{-0.25}$       |
| 1016.718         | $1.35^{+0.25}_{-0.24}$       |
| 1016.728         | $1.31^{+0.25}_{-0.24}$       |
| 1016.738         | $1.24^{+0.22}_{-0.22}$       |
| 1016.748         | $1.26^{+0.25}_{-0.24}$       |
| 1016.758         | $1.25^{+0.23}_{-0.23}$       |
| 1016.768         | $1.25^{+0.24}_{-0.23}$       |
| 1016.778         | $1.2^{+0.21}_{-0.23}$        |
| 1016.788         | $1.3^{+0.25}_{-0.24}$        |
| 1016.798         | $1.21^{+0.22}_{-0.22}$       |
| 1016.808         | $1.34^{+0.26}_{-0.24}$       |
| 1016.818         | $1.3^{+0.25}_{-0.23}$        |
| 1016.828         | $1.23^{+0.25}_{-0.27}$       |
| 1016.838         | $1.29^{+0.25}_{-0.24}$       |
| 1016.848         | $1.27^{+0.24}_{-0.24}$       |
| 1016.858         | $1.33^{+0.25}_{-0.24}$       |
| 1016.868         | $1.29^{+0.24}_{-0.23}$       |
| 1016.878         | $1.28^{+0.25}_{-0.24}$       |
| 1016.888         | $1.33^{+0.26}_{-0.24}$       |
| 1016.898         | $1.47^{+0.29}_{-0.28}$       |
| 1016.908         | $1.31^{+0.24}_{-0.23}$       |
| 1016.918         | $1.26^{+0.23}_{-0.23}$       |
| 1016.928         | $1.28^{+0.24}_{-0.23}$       |
| 1016.938         | $1.31^{+0.26}_{-0.25}$       |
| 1016.948         | $1.31^{+0.25}_{-0.24}$       |
| 1016.958         | $1.33^{+0.26}_{-0.24}$       |
| 1016.968         | $1.25^{+0.24}_{-0.23}$       |
| 1016.978         | $1.2^{+0.2}_{-0.22}$         |
| 1016.988         | $1.28^{+0.27}_{-0.28}$       |
| 1016.998         | $1.32^{+0.25}_{-0.23}$       |
| 1017.008         | $1.37^{+0.27}_{-0.25}$       |
| 1017.018         | $1.35^{+0.26}_{-0.24}$       |

**Table 1** *continued***Table 1** (*continued*)

| Start freq. (Hz) | $h_0^{95\%} \times 10^{-25}$ |
|------------------|------------------------------|
| 1017.028         | $1.25^{+0.23}_{-0.23}$       |
| 1017.038         | $1.31^{+0.27}_{-0.27}$       |
| 1017.048         | $1.32^{+0.25}_{-0.24}$       |
| 1017.058         | $1.21^{+0.22}_{-0.23}$       |
| 1017.068         | $1.29^{+0.24}_{-0.24}$       |
| 1017.078         | $1.33^{+0.25}_{-0.23}$       |
| 1017.088         | $1.36^{+0.27}_{-0.25}$       |
| 1017.098         | $1.29^{+0.24}_{-0.22}$       |
| 1017.108         | $1.21^{+0.21}_{-0.22}$       |
| 1017.118         | $1.34^{+0.26}_{-0.25}$       |
| 1017.128         | $1.24^{+0.22}_{-0.23}$       |
| 1017.138         | $1.33^{+0.24}_{-0.22}$       |
| 1017.148         | $1.27^{+0.24}_{-0.23}$       |
| 1017.158         | $1.3^{+0.25}_{-0.24}$        |
| 1017.168         | $1.27^{+0.25}_{-0.24}$       |
| 1017.178         | $1.25^{+0.23}_{-0.22}$       |
| 1017.188         | $1.31^{+0.26}_{-0.24}$       |
| 1017.198         | $1.23^{+0.28}_{-0.31}$       |
| 1017.208         | $1.3^{+0.22}_{-0.22}$        |
| 1017.218         | $1.24^{+0.23}_{-0.23}$       |
| 1017.228         | $1.26^{+0.24}_{-0.23}$       |
| 1017.238         | $1.2^{+0.21}_{-0.22}$        |
| 1017.248         | $1.2^{+0.22}_{-0.23}$        |
| 1017.258         | $1.25^{+0.24}_{-0.23}$       |
| 1017.268         | $1.23^{+0.24}_{-0.25}$       |
| 1017.278         | $1.2^{+0.22}_{-0.23}$        |
| 1017.288         | $1.24^{+0.23}_{-0.23}$       |
| 1017.298         | $1.28^{+0.25}_{-0.24}$       |
| 1017.308         | $1.2^{+0.23}_{-0.25}$        |
| 1017.318         | $1.21^{+0.23}_{-0.24}$       |
| 1017.328         | $1.34^{+0.25}_{-0.23}$       |
| 1017.338         | $1.24^{+0.29}_{-0.31}$       |
| 1017.348         | $1.3^{+0.25}_{-0.24}$        |
| 1017.358         | $1.3^{+0.25}_{-0.23}$        |
| 1017.368         | $1.24^{+0.23}_{-0.23}$       |
| 1017.378         | $1.33^{+0.25}_{-0.23}$       |
| 1017.388         | $1.38^{+0.27}_{-0.25}$       |
| 1017.398         | $1.27^{+0.27}_{-0.28}$       |
| 1017.408         | $1.28^{+0.24}_{-0.23}$       |
| 1017.418         | $1.29^{+0.25}_{-0.23}$       |
| 1017.428         | $1.22^{+0.21}_{-0.22}$       |
| 1017.438         | $1.31^{+0.26}_{-0.25}$       |

## REFERENCES

Abbott, B. P., Abbott, R., Abbott, T. D., et al. 2019,  
PhRvD, 99, 122002, doi: [10.1103/PhysRevD.99.122002](https://doi.org/10.1103/PhysRevD.99.122002)
